# Supplementary material for: Order-optimal Joint Transmission and Identification in Massive Multi-User MIMO via Group Testing
Source: arXiv:2210.00421 source file (2023-01-18)
Supplement: Supplementary file 1 [file Misc.tex]

\subsection{Choosing $\gamma$}
Unlike other works related to GT, the BAC channel's parameters can be, in hindsight, selected.
This discrete channel is a direct function of $p$ (recall that $J_i$ is also a function of $p$) and $\gamma$.
Furthermore, we can transmit using any power we like as long as it meets the power constraint.
In this subsection we present different choices to pick $\gamma$ and $p$.

\subsubsection{Bit Error Minimizer}
As we introduced earlier when calculating $q_{01}$ and $q_{10}$, $\gamma$ defines a trade-off between $q_{01}$ and $q_{10}$.
We can calculate the error probability of our decision rule:
\begin{align}
    \nonumber
    p_e
    &=
    \sum_{j=0}^K \mathbb{P}(J_i = j)\cdot \mathbb{P}(\text{bit flips}|J_i = j)
    \\\nonumber
    &=
    \sum_{j=0}^K \binom{K}{j}p^j(1-p)^{K-j}\mathbb{P}(\text{bit flips}|J_i = j)
    \\\label{eq:CharaErr_AvgErrDecisionRule}
    &=
    (1-p)^K q_{01} + (1-(1-p)^K) q_{10}
\end{align}
A suitable choice of $\gamma$ can be a minimizer of the error probability per antenna, $p_e$.
I.e., the solution to:
\begin{align}
    \begin{aligned}
        \min_{p, \gamma \in \mathbb{R}}  \quad & (1-p)^K q_{01} + (1-(1-p)^K) q_{10}
        \\
        \textrm{s.t.} \quad & 
        \begin{cases}
            0 \leq \gamma \\
            0 \leq p \leq \frac{1}{2}
        \end{cases}
    \end{aligned}
\end{align}
Notice that $p_e$'s curvature in $\gamma$ or $p$ is ambiguous.

\subsubsection{BAC Capacity Maximizer}
$q_{01}$ and $q_{10}$ define some BAC as presented in figure \ref{fig:CharaErrBAC}.
Intuitively, the capacity measures the amount of information bits received per antenna.
Maximizing this quantity minimizes the number of antennas necessary for our scheme (by theorem \ref{eq:ConverseMrBound} or corollary \ref{eq:ConverseMrBoundWithC}), so a valid choice of $\gamma$ is:
\begin{align}
    \begin{aligned}
        \max_{p, \gamma \in \mathbb{R}}  \quad & \capacity{BAC(q_{01},q_{10})}
        \\
        \textrm{s.t.} \quad & 
        \begin{cases}
            0 \leq \gamma \\
            0 \leq p \leq \frac{1}{2}
        \end{cases}
    \end{aligned}
\end{align}
We provide a contour plot of the channel capacity as a function of $\rho$ and $\gamma$ in figure \ref{fig:CharaErrBAC_contour}.
\begin{figure}[!htbp]
    \centering
    \begin{tikzpicture}[x=1pt, y=1pt, yscale=-1, xscale=1]
        % Nodes
        \node (X) at (55,72.5) {$X$};
        \node (Y) at (265,72.5) {$Y$};
        \node (0Orig) at (65,30) {$0$};
        \node (1Orig) at (65,115) {$1$};
        \node (0Chan) at (255,30) {$0$};
        \node (1Chan) at (255,115) {$1$};
        
        % Edges
        \draw[-stealth]    (0Orig) -- (0Chan) node[midway, above] {$1-q_{01}$};
        \draw[-stealth]    (1Orig) -- (1Chan)  node[midway, below] {$1-q_{10}$};
        \draw[-stealth]    (0Orig) -- (1Chan)  node[near start, below] {$q_{01}$};
        \draw[-stealth]    (1Orig) -- (0Chan) node[near start, above] {$q_{10}$};
    \end{tikzpicture}
    \caption{BAC with transition probabilities $q_{01}$ and $q_{10}$.
    When a bit is transmitted, it can flip into the other bit, and this probability depends on the transmitted bit.
    }
    \label{fig:CharaErrBAC}
\end{figure}
\begin{figure}[!htbp]
    \centering
    \includegraphics[scale=0.17]{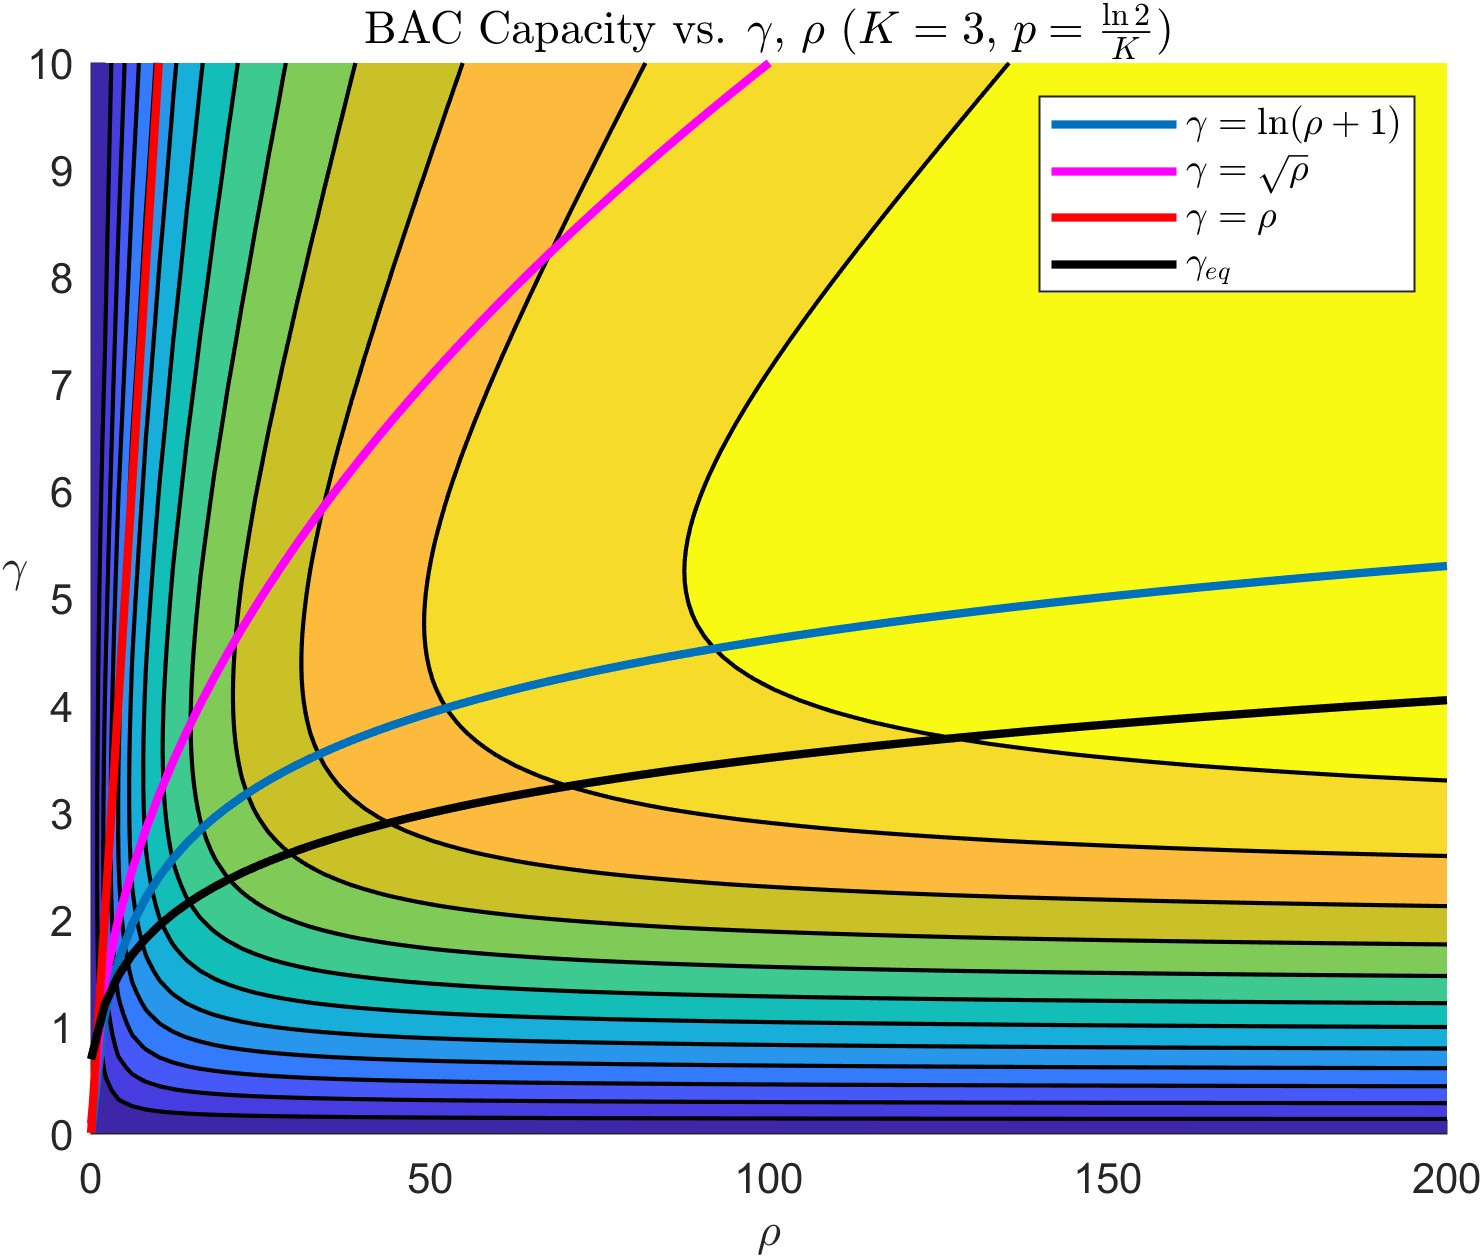}
    \caption{
    Contour plot of the BAC capacity for $N_0 = 1$, $K = 3$ and $p = \frac{\ln 2}{K}$.
    Brighter color (closer to yellow) implies higher capacity.
    As $\rho$ increases, a lower $\gamma$ is required to get closer to one bit per antenna.
    The red line corresponds to $\gamma = \rho$, and the capacity for this choice is greatly lower than any other choice of $\gamma$.
    The curve $\gamma = \ln (\rho + 1)$ is close to the optimal choice of $\gamma$ (as it is closer than any other choice to the nearest point per contour line).
    The black curve is corresponds to $\gamma_{eq}$, the equalizer of $q_{01}$ and $q_{10}$.
    }
    \label{fig:CharaErrBAC_contour}
\end{figure}

\subsubsection{Reduction to Solved Cases}
\label{subsubsect:CoMa_reduce}
Assume we solve $q_{01} = q_{10}$ for $\gamma$ when $p = \frac{0.5}{K}$ to obtain $\gamma_{eq}$.
When using $\gamma_{eq}$, our MAC problem can be reduced to Chan et al.'s GT problem with symmetric noise (\cite{CoMa2}), so $M_r = O(K\log N)$.

\subsection{Sufficient Condition for Vanishing Error Probabilities}
Theorems \ref{theo:CoMa_pMD_ub} and \ref{theo:CoMa_pFA_ub} produce the following corollaries:
\begin{corollary}[Sufficient Condition for Vanishing Miss-Detection Probability]
\label{theo:CoMa_pMD_suff_con}
Assume $0 < \Delta$.
If $M_r\cdot p \cdot (q_{10}\Delta)^2\to\infty$ when $N\to\infty$ then $p_{MD}\to0$.
\end{corollary}

\begin{corollary}[Sufficient Condition for Vanishing False Alarm Probability]
\label{theo:CoMa_pFA_suff_con}
Assume $0 < \Delta < \frac{p_0}{q_{10}}-1$.
If $M_r\cdot p \cdot (p_0 - q_{10}(\Delta+1))^2\to\infty$ when $N\to\infty$ then $p_{FA}\to0$.
\end{corollary}

Note that $\Delta$ is a fine-tuning parameter of the Noisy CoMa algorithm, affected by choice of $\gamma$.
The choice of $\gamma$ depends on the SNR, $\rho$.
In other words, if $\rho$ is constant, then so are $\gamma$ and $\Delta$.
This implies that $q_{10}$, $q_{01}$ and $p_0$ are constants too.
Hence, both errors ($p_{MD}$ and $p_{FA}$) tend to zero if $M_r\cdot p\to\infty$ (assuming $\Delta$ satisfies the conditions from corollary \ref{theo:CoMa_pFA_suff_con}).
