# Supplementary material for: Order-optimal Joint Transmission and Identification in Massive Multi-User MIMO via Group Testing
Source: arXiv:2210.00421 source file (2023-01-18)
Supplement: Supplementary file 2 [file Proofs_for_short.tex]

\subsection{Proof of Theorems \ref{eq:CharaErr_q01} and \ref{eq:CharaErr_q10}}
% \ref{lem:CharaErr_yi2_dist}
\label{appendix:proof_CharaErr_yi2_dist}
Denote the number of users targeting the $i^{\mathrm{th}}$ antenna $J_i$.
When each transmitter has a random codebook generated by i.i.d. coin tosses with probability $p$ for '1', $J_i\sim \text{Bin}(K, p)$.
By their definition, 
\begin{align}
    \label{eq:CharaErr_q01_def}
    q_{01}
    &\triangleq
    \mathbb{P}(|[\underline{y}]_i|^2\geq N_0\cdot\gamma\ |\ J_i = 0)
    \\\label{eq:CharaErr_q10_def}
    q_{10}
    &\triangleq
    \mathbb{P}(|[\underline{y}]_i|^2\leq N_0\cdot\gamma\ |\ J_i \geq 1)
\end{align}
Before calculating the error probabilities, we would like to introduce a helpful lemma about the distribution of $|[\underline{y}]_i|^2 \big| J_i$:
\begin{lemma}
\label{lem:CharaErr_yi2_dist}
Assume each transmitter uses ZFBF with no optimizations to the power allocation.
Then:
\begin{align}
    \nonumber
    |[\underline{y}]_i|^2 \big| J_i
    \sim
    \mathrm{Exp}\bigg(
        \frac{1}{J_i\cdot P+N_0}
    \bigg)
\end{align}
\end{lemma}
\begin{proof}
Each transmitter uses ZFBF by taking an arbitrary normalized vector from the nullspace of some submatrix from their channel matrix.
Afterward, the vector is amplified by $\sqrt{P}$.
Hence, from the rotational invariance of the CGRVs, each user contributes a zero-mean $P$-variance CGRV.
Since all users are independent and $J_i$ users target the $i^{\text{th}}$ antenna, these RVs are i.i.d. and summed with the additive noise.
As a result, $[\underline{y}]_i$ is a CGRV as a linear combination of CGRVs.
I.e., $[\underline{y}]_i\sim \mathcal{CN}(0, J_i\cdot P + N_0)$.
By the Random Variable Transformation Theorem, we obtain the desired result.

For completeness, we attach the full calculation;
Denote $\sigma^2 \triangleq \frac{J_i\cdot P + N_0}{2}$.
$[\underline{y}]_i\sim \mathcal{CN}(0, 2\sigma^2)$, so $\Re([\underline{y}]_i)\overset{d}{=}\Im([\underline{y}]_i)\sim\mathcal{N}(0, \sigma^2)$.
We are interested in the distribution of $W\triangleq|[\underline{y}]_i^2| = \Re([\underline{y}]_i)^2 + \Im([\underline{y}]_i)^2$.
The proof has two steps - first, we calculate $Z \triangleq \sqrt{W}$'s CDF.
Then, we show that $W\sim\mathrm{Exp}(\frac{1}{2\sigma^2})$ by the Random Variable Transformation Theorem:
\begin{align}
    F_{Z}(z)
    &=
    \mathbb{P}(Z \leq z)
    \\
    &=
    \mathbb{P}\big(\sqrt{\Re([\underline{y}]_i)^2 + \Im([\underline{y}]_i)^2} \leq z\big)
    \\
    &\underset{(a)}{=}
    \iint\limits_{\sqrt{x^2+y^2}\leq z} \frac{1}{2\pi \sigma^2}\exp\bigg\{-\frac{x^2+y^2}{2\sigma^2}\bigg\} dx dy
    \\
    &\underset{(b)}{=}
    \int_{0}^z\int_{0}^{2\pi} \frac{r}{2\pi \sigma^2}\exp\bigg\{-\frac{r^2}{2\sigma^2}\bigg\} d\theta dr
    \\
    &\underset{(c)}{=}
    \int_{0}^z \frac{r}{\sigma^2}\exp\bigg\{-\frac{r^2}{2\sigma^2}\bigg\} dr
\end{align}
In (a), we recalled that $\Re([\underline{y}]_i)$ and $\Im([\underline{y}]_i)$ are independent from the definition of CGRV, so they are jointly Gaussian.
In (b), we changed the integration variables from $x$ and $y$ to $r\cos{\theta}$ and $r\sin{\theta}$, respectively.
The Jacobian, in this case, is $r$.
Step (c) is justified by noticing that the integrand is not a function of $\theta$.

By deriving the CDF, we obtain that $Z$'s PDF is:
\begin{align}
    \label{eq:CharaErr_Z_PDF}
    f_{Z}(z) = 
    \begin{cases}
        \frac{z}{\sigma^2} \cdot e^{-\frac{z^2}{2\sigma^2}} & z\geq 0 \\
        0 & z < 0
    \end{cases}
\end{align}
When $w < 0$, there is no solution to $w = z^2$ (as a function of $z$).
Hence, $f_W(w) = 0$ for any $w < 0$.
In any other case, $z = \pm\sqrt{w}$.
Now we are ready to calculate $W$'s PDF:
\begin{align}
    f_{W}(w)
    &\underset{(a)}{=}
    \frac{f_{Z}(-\sqrt{w})}{|\frac{\partial w}{\partial z}|} + \frac{f_{Z}(\sqrt{w})}{|\frac{\partial w}{\partial z}|}
    \\
    &\underset{(b)}{=}
    \frac{1}{2\sqrt{w}}\big(
        f_{Z}(-\sqrt{w}) + f_{Z}(\sqrt{w})
    \big)
    \\
    &\underset{(c)}{=}
    \frac{1}{2\sqrt{w}}\bigg(
        \frac{\sqrt{w}}{\sigma^2} \cdot e^{-\frac{w}{2\sigma^2}}
        +
        0
    \bigg)
    \\
    &=
    \frac{1}{2\sigma^2} \cdot e^{-\frac{w}{2\sigma^2}}
\end{align}
Step (a) is the Random Variable Transformation Theorem.
In step (b), we calculate $|\frac{\partial w}{\partial z}| = 2 |z| = 2\sqrt{w}$.
We substituted (\ref{eq:CharaErr_Z_PDF}) in step (c).
Finally, $W$'s PDF is given by:
\begin{align}
    \label{eq:CharaErr_W_PDF}
    f_{W}(w) = 
    \begin{cases}
        \frac{1}{2\sigma^2} \cdot e^{-\frac{w}{2\sigma^2}} & w\geq 0 \\
        0 & w < 0
    \end{cases}
\end{align}
Which is the PDF of an exponentially distributed random variable with parameter $\frac{1}{2\sigma^2}$.
I.e., $|[\underline{y}]_i^2|\sim\mathrm{Exp}(\frac{1}{J_i\cdot P + N_0})$.
\end{proof}

Now, we can straightforwardly calculate the crossover probabilities, starting with $q_{01}$:
\begin{align}
    q_{01}
    &\underset{(a)}{=}
    \mathbb{P}(|[\underline{y}]_i|^2\geq N_0\cdot\gamma\ |\ J_i = 0)
    \\
    &\underset{(b)}{=}
    \int_{N_0\cdot\gamma}^\infty \frac{1}{N_0}e^{-\frac{t}{N_0}} dt
    \\
    &=
    e^{-\gamma}
\end{align}
Transition (a) used (\ref{eq:CharaErr_q01_def}), whereas (b) used lemma \ref{lem:CharaErr_yi2_dist}.
Calculating $q_{10}$:
\begin{align}
    q_{10}
    &\underset{(a)}{=}
    \mathbb{P}(|[\underline{y}]_i|^2\leq N_0\cdot\gamma\ |\ J_i \geq 1)
    \\
    &\underset{(b)}{=}
    \mathbb{E}_{J_i\geq1}[\mathbb{P}(|[\underline{y}]_i|^2\leq N_0\cdot\gamma\ |\ J_i)\ |\ J_i]
    \\
    &\underset{(c)}{=}
    \sum_{j=1}^K \binom{K}{j}\frac{p^j(1-p)^{K-j}}{1-(1-p)^K} \cdot\mathbb{P}(|y_i|^2\leq N_0\cdot\gamma\ |\ J_i=j)
    \\
    &\underset{(d)}{=}
    \sum_{j=1}^K \binom{K}{j}\frac{p^j(1-p)^{K-j}}{1-(1-p)^K}\bigg(1 - \exp\bigg\{-\frac{N_0\cdot\gamma}{j \cdot P + N_0}\bigg\}\bigg)
    \\
    &=
    \sum_{j=1}^K \binom{K}{j}\frac{p^j(1-p)^{K-j}}{1-(1-p)^K}\bigg(1 - \exp\bigg\{-\frac{\gamma}{j \cdot \rho + 1}\bigg\}\bigg)   
\end{align}
In (a), we used (\ref{eq:CharaErr_q10_def}) and (b) used the Smoothing Theorem.
In (c), we write the conditional expectation explicitly.
Note that the term $\frac{1}{1-(1-p)^K}$ is used to convert the event $J_i\geq1$ into a proper probability measure.
Step (d) used lemma \ref{lem:CharaErr_yi2_dist}.
The last step normalized the term inside the exponent by $N_0$ defining $\rho \triangleq \frac{P}{N_0}$.

\subsection{Proof of Theorem \ref{theo:CoMa_pMD_to0_suff_cond}}
\label{appendix:proof_CoMa_pMD_to0_suff_cond}
We define how Noisy CoMa obtains messages from $\underline{Y}$:
\begin{definition}[Noisy CoMa Decision Criterion]
\label{def:CoMa_jWordDecisionRule}
Fix $\Delta > 0$.
Denote $\mathrm{supp}(\underline{x})$ as the set of indices where $\underline{x}$ has non-zero components.
Let $\mathcal{T}_j\triangleq|\mathrm{supp}(\underline{c}_j)|$ and $\mathcal{S}_j\triangleq|\mathrm{supp}(\underline{c}_j)\cap\mathrm{supp}(\underline{Y})|$.
Noisy CoMa's declares that $\underline{c}_j$ has been transmitted is if and only if $\mathcal{S}_j \geq \mathcal{T}_j(1-q_{10}(\Delta+1))$.
\end{definition}
For simplicity, we shall use $N$ for the total number of codewords rather than the number of users.
I.e., $N = N'\cdot C$.
\begin{theorem}
    \label{theo:CoMa_pMD_ub}
    The probability of missing at least one true codeword is bounded from above by:
    \begin{align}
        \nonumber
        p_{MD} \leq K\cdot \exp\bigg\{-M_r\cdot p \cdot\big(1-e^{-2(q_{10}\Delta)^2}\big)\bigg\}
    \end{align}
\end{theorem}
\begin{proof}
    \begin{align}
        p&_{MD}
        \underset{(a)}{\leq}
        K\cdot \sum_{i=0}^{M_r} \mathbb{P}(\mathcal{T}_1 = i)\cdot \mathbb{P}(\mathcal{S}_1 < \mathcal{T}_1 (1-q_{10}(\Delta+1)))
        \\
        &\underset{(b)}{=}
        K\cdot\sum_{i=0}^{M_r} \binom{M_r}{i}p^i(1-p)^{M_r-i}
        \\\nonumber&\quad\cdot\mathbb{P}(\mathcal{T}_1 < i(1-q_{10}(\Delta+1)))
        \\
        &\underset{(c)}{=}
        K\cdot\sum_{i=0}^{M_r} \binom{M_r}{i}p^i(1-p)^{M_r-i}
        \\\nonumber
        &\ \ \ \ \cdot\sum_{l=i-i(1-q_{10}(\Delta+1))}^i \binom{i}{l} q_{10}^i (1-q_{10})^{i-l}
        \\
        &\underset{(d)}{\leq}
        K\cdot \sum_{i=0}^{M_r} \binom{M_r}{i}p^i(1-p)^{M_r-i}
        \cdot e^{-2i(q_{10}\Delta)^2}
        \\
        &\underset{(e)}{=}
        K\cdot\big(1-p+p e^{-2(q_{10}\Delta)^2}\big)^{M_r}
        \\
        &\underset{(f)}{\leq}
        K\cdot \exp\bigg\{-p\big(1-e^{-2(q_{10}\Delta)^2}\big)\bigg\}^{M_r}
        \\
        &=
        K\cdot \exp\bigg\{-M_r\cdot p\cdot\big(1-e^{-2(q_{10}\Delta)^2}\big)\bigg\}
    \end{align}
    In (a), we used the union bound.
    (b) is derived from the random codebook construction where $\mathcal{S}_1\sim\text{Bin}(M_r, p)$.
    In (c), we used the fact that the local decision rule is identical among the antennas, so the probability for bit flips is symmetric (the number of flipped bits is binomially distributed with parameters $M_r$, $q_{10}$).
    Additionally, we used the binomial distribution's symmetry\footnote{$F(k; n, p) = F(n-k; n, 1-p)$}.
    We used Hoeffding bound\footnote{often called Chernoff bound}, $F(k; n, p) \leq \exp\{-2n(p-\frac{k}{n})^2\}$ and $p-\frac{k}{n} > 0$, in (d).
    (e) used the binomial theorem to combine the sum of products into a power of a sum.
    In (f) we used the Taylor Expansion of $\exp\{-x(1-a)\}$ at $x_0 = 0$.
\end{proof}
Now we are ready to prove Theorem \ref{theo:CoMa_pMD_to0_suff_cond}:
\begin{align}
    p_{MD}
    &\underset{(a)}{\leq}
    K\cdot \exp\bigg\{-M_r\cdot p \cdot\big(1-e^{-2(q_{10}\Delta)^2}\big)\bigg\}
    \\
    &\underset{(b)}{=}
    K\cdot \exp\bigg\{-\beta_1 \cdot K\log N\cdot p\cdot\big(1-e^{-2(q_{10}\Delta)^2}\big)\bigg\}
    \\
    &\underset{(c)}{\leq}
    K \exp\bigg\{-\frac{(1+\delta) K\log N\cdot p\big(1-e^{-2(q_{10}\Delta)^2}\big)}{\alpha\big(1-e^{-2(q_{10}\Delta)^2}\big)\log e} \bigg\}
    \\
    &\underset{(d)}{=}
    K \exp\bigg\{-\frac{(1+\delta)\cdot K\log N\cdot \frac{\alpha}{K}}{\alpha\log e} \bigg\}
    \\
    &\underset{(e)}{=}
    K \exp\big\{-(1+\delta) \ln N \big\}    
    \\
    &\underset{(f)}{=} K \cdot N^{-(1+\delta)}
    \leq N \cdot N^{-(1+\delta)} = N^{-\delta}
\end{align}
(a) used Theorem \ref{theo:CoMa_pMD_ub}.
In (b), we utilized Theorem \ref{theo:CoMa_pMD_to0_suff_cond}'s conditions.
(c) replaced $\beta_1$ with its lower bound (from the theorem's conditions), and in (d),  we reduced the fraction and replaced $p=\frac{\alpha}{K}$.
(e) used algebraic manipulation using logarithmic identities, and (f) used the logarithm's definition.

\subsection{Proof of Theorem \ref{theo:CoMa_pFA_to0_suff_cond}}
\label{appendix:proof_CoMa_pFA_to0_suff_cond}
Similar to the previous theorem, we bound $p_{FA}$:
\begin{theorem}
    \label{theo:CoMa_pFA_ub}
    Assume $\Delta < \frac{p_0}{q_{10}}-1$.
    The probability of declaring at least one false codeword is bounded from above by:
    \begin{align}
        \nonumber
        p_{FA} \leq (N-K)
        \exp\bigg\{-M_r\cdot p\cdot \big(1-e^{-2(p_0-q_{10}(\Delta+1))^2}\big)\bigg\}
    \end{align}
\end{theorem}
\begin{proof}
    \begin{align}
        p&_{FA}
        \leq
        (N-K)\cdot\sum_{i=0}^{M_r} \mathbb{P}(\mathcal{T}_1 = i)
        \\\nonumber&\quad\cdot \mathbb{P}(\mathcal{S}_1 \geq \mathcal{T}_1 (1-q_{10}(\Delta+1)))
        \\
        &=
        (N-K)\cdot\sum_{i=0}^{M_r} \binom{M_r}{i}p^i(1-p)^{M_r-i}
        \\\nonumber
        &\ \ \ \ 
        \cdot\sum_{l=i(1-q_{10}(\Delta+1))}^i \binom{i}{l} p_1^i (1-p_1)^{i-l}
        \\
        &\underset{(a)}{\leq}
        (N-K)\cdot \sum_{i=0}^{M_r} \binom{M_r}{i}p^i(1-p)^{M_r-i}
        \\\nonumber&\quad\cdot e^{-2i(1-p_1-q_{10}(\Delta+1))^2}
        \\
        &\underset{(b)}{=}
        (N-K)\cdot \sum_{i=0}^{M_r} \binom{M_r}{i}p^i(1-p)^{M_r-i} e^{-2i(p_0-q_{10}(\Delta+1))^2}
        \\
        &=
        (N-K)\cdot \big(1-p+p e^{-2(p_0-q_{10}(\Delta+1))^2}\big)^{M_r}
        \\
        &\leq
        (N-K)\cdot
        \exp\bigg\{-M_r\cdot p\cdot \big(1-e^{-2(p_0-q_{10}(\Delta+1))^2}\big)\bigg\}
    \end{align}
    In (a) we used Hoeffding bound like in the proof of Theorem \ref{theo:CoMa_pMD_ub}, which is applicable due to $\Delta < \frac{p_0}{q_{10}}-1$.
    We replace $1-p_1 = p_0$ in (b).
    Any other transition is identical to the proof of Theorem \ref{theo:CoMa_pMD_ub}.
\end{proof}
Now we prove Theorem \ref{theo:CoMa_pFA_to0_suff_cond}:
\begin{align}
    p_{FA}
    &\underset{(a)}{\leq}
    (N-K)
    \exp\bigg\{-M_r\cdot p\cdot \big(1-e^{-2(p_0-q_{10}(\Delta+1))^2}\big)\bigg\}
    \\
    &\underset{(b)}{=}
    (N-K) \exp\bigg\{-\beta_2 K\log N\cdot p
    \\\nonumber
    &\ \ \ \ \cdot \big(1-e^{-2(p_0-q_{10}(\Delta+1))^2}\big)\bigg\}
    \\
    &\underset{(c)}{\leq}
    N\cdot \exp\bigg\{-\frac{(1+\delta)K\log N\cdot p}{\alpha \big(1-e^{-2(p_0-q_{10}(\Delta+1))^2}\big)\log e}
    \\\nonumber
    &\ \ \ \ \cdot \big(1-e^{-2(p_0-q_{10}(\Delta+1))^2}\big)\bigg\}
    \\
    &=
    N\cdot \exp\big\{-(1+\delta)\ln N\big\}
    \leq N^{-\delta}
\end{align}
In (a) we used theorem \ref{theo:CoMa_pFA_ub}.
In both (b) and (c) we used theorem \ref{theo:CoMa_pFA_to0_suff_cond}'s conditions.
The rest is similar to the proof of theorem \ref{theo:CoMa_pMD_to0_suff_cond}.

\subsection{Proof of Theorem \ref{theo:CoMa_b_opt_prob_equiv}}
\label{appendix:proof_CoMa_b_opt_prob_equiv}
First, we simplify $\frac{p_0}{q_{10}}-1$:
\begin{align}
    \nonumber
    \frac{p_0}{q_{10}} -1
    &=
    \frac{(1-p)^K (1-q_{01}) + (1-(1-p)^K)q_{10}}{q_{10}} - 1
    \\\label{eq:CoMa_Delta_up_simp}
    &=
    (1-p)^K\cdot\frac{1-q_{01}-q_{10}}{q_{10}}
\end{align}
Now, we convert the problem in (\ref{eq:CoMa_b_opt_prob_orig}) to a minimization problem by removing the dependence on $\Delta$: 
\begin{lemma}
\label{eq:CoMa_b_opt_prob_orig_reduce_minimax}
The objective function in (\ref{eq:CoMa_b_opt_prob_orig}) can be re-written as follows:
\begin{align}
    \nonumber
    \frac{(1+\delta)\ln 2}{\alpha\big(1-\exp\{-\frac{1}{2}(1-p)^{2K}(1-q_{10}-q_{01})^2\}\big)}
\end{align}
\end{lemma}
\begin{proof}
Derive $\beta_i$ by $\Delta$:
\begin{align}
    \frac{\partial\beta_1}{\partial \Delta}
    &=
    -\frac{4 q_{10}^2 e^{-2(q_{10}\Delta)^2}\Delta}{(\cdot)^2} \leq 0 \ \forall \Delta\geq0
    \\
    \frac{\partial\beta_2}{\partial \Delta}
    &=
    \frac{4q_{10}e^{-2(p_0-q_{10}(\Delta+1))^2}(p_0-q_{10}(\Delta+1))}{(\cdot)^2}
\end{align}
The last term is non-negative as long as $\Delta\leq \frac{p_0}{q_{10}}-1$.
Hence, $\beta_1$ decrease with $\Delta$ whereas $\beta_2$ increase in $\Delta$.
In other words, the minimax problem would pick the equalizer:
\begin{align}
    \Delta^*
    &=
    \frac{1}{2}\bigg(\frac{p_0}{q_{10}}-1\bigg)
\end{align}
Putting $\Delta^*$ and (\ref{eq:CoMa_Delta_up_simp}) back into $\beta_1=\beta_2$ results in the following term inside the exponent:
\begin{align}
    q_{10}\cdot \frac{1}{2}\bigg(\frac{p_0}{q_{10}}-1\bigg)
    &=
    \frac{1}{2}(1-p)^K(1-q_{01}-q_{10})
\end{align}
\end{proof}
We shall henceforth name the objective function $\beta = (1+\delta)\cdot\beta(\gamma, \alpha)$.
Now, we shall prove that the solution must be an interior point of the rectangle $[0,\frac{K}{2}]\times[0,\infty)$:
\begin{lemma}
\label{eq:CoMa_b_opt_prob_orig_reduce_weak_ineq}
All strong inequalities in (\ref{eq:CoMa_b_opt_prob_orig}) can be written with weak inequalities.
\end{lemma}
\begin{proof}
We'll show that each time some variable meets its strong inequality then either $\beta_1\to\infty$ or $\beta_2\to\infty$.
When $\gamma = 0$, $q_{10} = 0$ and $\beta_1\to\infty$.
The same occurs when $\Delta = 0$.
When $\Delta = \frac{p_0}{q_{10}}-1$ then $\beta_2\to\infty$.
When $\alpha = 0$ both $\beta_i\to\infty$.
Hence, we can replace the strong inequalities with weak inequalities as we do not introduce new solutions to the optimization problem.
\end{proof}
We are left with proving that $\alpha = \frac{K}{2}$ is not a solution to the optimization problem.
To do this, we show that there always is an interior point with a lower objective value.
Hence, we define the following two quantities:

\begin{definition}
\label{def:CoMa_gamma1}
For any fixed $p$, we define $\gamma_1$ to be the solution to:
\begin{align}
    \nonumber
    e^{-\gamma}
    =
    \sum_{j=1}^K \binom{K}{j}\frac{p^j (1-p)^{K-j}}{1-(1-p)^K}
    \cdot 
    \frac{\exp\big\{\frac{-\gamma}{j\rho +1}\big\}}{j\rho +1}
\end{align}
\end{definition}

\begin{definition}
\label{def:CoMa_gamma2}
Let $\gamma_2$ be the solution to:
\begin{align}
    \nonumber
    e^{-\gamma}
    =
    \sum_{j=1}^K \binom{K}{j}\frac{1}{2^K-1}\cdot\frac{\exp\big\{\frac{-\gamma}{j\rho +1}\big\}}{j\rho +1}
\end{align}
\end{definition}
We want to show that $\gamma_1$, as an interior point, has a lower objective function than $\gamma_2$, a point on the boundary.

\begin{lemma}
\label{lem:CoMa_beta_trend_gamma1}
$\beta(\gamma_1)$ is increasing in $\gamma_1$, where $\gamma_1$ is as defined in definition \ref{def:CoMa_gamma1}.
\end{lemma}

\begin{proof}
Putting $\gamma_1$ in $g(\gamma,p)\triangleq(1-q_{01}-q_{10})$ yields:
\begin{align}
    g(\gamma_1,p)
    &=
    1
    -
    \sum_{j=1}^K
    \binom{K}{j}\frac{p^j (1-p)^{K-j}}{1-(1-p)^K}
    \cdot
    \bigg(
        \\\nonumber
        &\ \ \ \ 
        \frac{\exp\big\{\frac{-\gamma_1}{j\rho +1}\big\}}{j\rho +1}
        +1-
        \exp\bigg\{-\frac{\gamma_1}{j \rho + 1}\bigg\}
    \bigg)
    \\
    &=
    \sum_{j=1}^K
    \binom{K}{j}\frac{p^j (1-p)^{K-j}}{1-(1-p)^K}
    \cdot
    \frac{j\rho\cdot \exp\big\{\frac{-\gamma_1}{j\rho +1}\big\}}{j\rho +1}
\end{align}
$g(\gamma_1(p),p)$ is a sum of non-negative numbers, so $g(\gamma_1,p)\geq0$.
Furthermore, $\frac{\partial g}{\partial \gamma_1} \leq 0$.
Observe $\beta$'s derivative with respect to $\gamma_1$:
\begin{align}
    \frac{\partial\beta(\gamma_1)}{\partial\gamma_1}
    =
    -\frac{(1-p)^{2K}e^{(\cdot)} g(\gamma_1)\cdot \frac{\partial g}{\partial \gamma_1}}{\alpha\cdot (\cdot)^2} \geq 0 \ \forall\alpha > 0
\end{align}
\end{proof}

\begin{lemma}
\label{lem:CoMa_gamma1_lb}
\begin{align}
    e^{-\gamma_1}
    \geq
    \sum_{j=1}^K \binom{K}{j}\frac{1}{2^K-1}\cdot\frac{\exp\big\{\frac{-\gamma_1}{j\rho +1}\big\}}{j\rho +1}
\end{align}
With equality if and only if $p=0.5$.
\end{lemma}

\begin{proof}
Observing $\gamma_1 = \gamma_1(p)$, we have $\gamma_2 = \gamma_1(0.5)$.
\begin{align}
    e^{-\gamma_1}
    &\underset{(a)}{=}
    \sum_{j=1}^K \binom{K}{j}\frac{p^j (1-p)^{K-j}}{1-(1-p)^K}
    \cdot 
    \frac{\exp\big\{\frac{-\gamma_1}{j\rho +1}\big\}}{j\rho +1}
    \\
    &\underset{(b)}{=}
    \sum_{j=\floor{\frac{K-1}{2}}}^K \binom{K}{j}\frac{p^j (1-p)^{K-j}}{1-(1-p)^K}
    \cdot 
    \frac{\exp\big\{\frac{-\gamma_1}{j\rho +1}\big\}}{j\rho +1}
    \\\nonumber
    &\ \ \ \ +
        \sum_{j=1}^{\floor{\frac{K-1}{2}}-1} \binom{K}{j}\frac{p^j (1-p)^{K-j}}{1-(1-p)^K}
        \cdot 
        \frac{\exp\big\{\frac{-\gamma_1}{j\rho +1}\big\}}{j\rho +1}
    \\
    &\underset{(c)}{\geq}
    \sum_{j=\floor{\frac{K-1}{2}}}^K \binom{K}{j}\frac{1}{2^K-1}
    \cdot 
    \frac{\exp\big\{\frac{-\gamma_1}{j\rho +1}\big\}}{j\rho +1}
    \\\nonumber
    &\ \ \ \ +
        \sum_{j=1}^{\floor{\frac{K-1}{2}}-1} \binom{K}{j}\frac{p^j (1-p)^{K-j}}{1-(1-p)^K}
        \cdot 
        \frac{\exp\big\{\frac{-\gamma_1}{j\rho +1}\big\}}{j\rho +1}    
    \\
    &\underset{(d)}{=}
    \sum_{j=1}^K \binom{K}{j}\frac{1}{2^K-1}
    \cdot 
    \frac{\exp\big\{\frac{-\gamma_1}{j\rho +1}\big\}}{j\rho +1}
    \\\nonumber
    &\ \ \ \ +
        \sum_{j=1}^{\floor{\frac{K-1}{2}}-1} \binom{K}{j}\bigg(\frac{p^j (1-p)^{K-j}}{1-(1-p)^K}
        -
        \frac{1}{2^K-1}
        \bigg)
        \\\nonumber
        &\quad\quad\cdot
        \frac{\exp\big\{\frac{-\gamma_1}{j\rho +1}\big\}}{j\rho +1}
    \\
    &\underset{(e)}{\geq}
    \sum_{j=1}^K \binom{K}{j}\frac{1}{2^K-1}
    \cdot 
    \frac{\exp\big\{\frac{-\gamma_1}{j\rho +1}\big\}}{j\rho +1}
\end{align}
In (a) we used definition \ref{def:CoMa_gamma1}.
We separated the sum in (b), and used $p$'s limited range ($p\in[0,1]$) in (c).
We have added and subtracted the same term in (d), whereas in (e), we discarded non-negative terms due to $p$'s range.
If $\gamma_1 = \gamma_2$, then we have equality from definition \ref{def:CoMa_gamma2}.
\end{proof}

\begin{corollary}
\label{cor:CoMa_gamma1_opt}
$\beta(\gamma_2)\geq\beta(\gamma_1)$
\end{corollary}

\begin{proof}
$\gamma_2$ is the maximizer of the lower bound in lemma \ref{lem:CoMa_gamma1_lb}.
In other words:
\begin{align}
    e^{-\gamma_1} \geq e^{-\gamma_2}
\end{align}
By taking $\ln(\cdot)$ from both sides we have $\gamma_2\geq\gamma_1$.
Using lemma \ref{lem:CoMa_beta_trend_gamma1} gives us the desired result.
\end{proof}

Now, after showing that the solution must be an interior point, we are ready to show that a solution exists:
\begin{lemma}
\label{lem:CoMa_obj_convex_in_gamma_suff}
The objective function in lemma \ref{eq:CoMa_b_opt_prob_orig_reduce_minimax} is convex in $\gamma$.
\end{lemma}

\begin{proof}
% We'll start with convexity w.r.t. $\gamma$.
$\beta(\gamma)$ is convex in $\gamma$ if and only if:
\begin{align}
    2\bigg(\frac{\partial f}{\partial\gamma}\bigg)^2
    -
    f(\gamma)\cdot\frac{\partial^2 f}{\partial\gamma^2}
    \geq
    0
\end{align}
By dividing by non-zero positive quantities, the above condition is simplified to:
\begin{align}
    \label{eq:CoMa_b_convex_gamma_cond}
    &\bigg(
        e^{\frac{1}{2}(1-p)^{2K}(1-q_{01}-q_{10})^2}+1
    \bigg)
    \cdot
    (1-p)^{2K}
    \cdot
    (1-q_{01}-q_{10})^2
    \\\nonumber
    &\ \ \ \ 
    \cdot
    \bigg(
        \frac{\partial q_{01}}{\partial\gamma}
        +
        \frac{\partial q_{10}}{\partial\gamma}
    \bigg)^2
    +
    \bigg(
        e^{\frac{1}{2}(1-p)^{2K}(1-q_{01}-q_{10})^2}-1
    \bigg)
    \\\nonumber
    &\ \ \ \ 
    \cdot
    \bigg[
        (
            1
            -
            q_{01}
            -
            q_{10}
        )
        \bigg(
            \frac{\partial^2 q_{01}}{\partial\gamma^2}
            +
            \frac{\partial^2 q_{10}}{\partial\gamma^2}
        \bigg)
        \\\nonumber&\quad
        -
        \bigg(
            \frac{\partial q_{01}}{\partial\gamma}
            +
            \frac{\partial q_{10}}{\partial\gamma}
        \bigg)^2
    \bigg]
    \geq 0
\end{align}
Rearranging both sides results in the following:
\begin{align}
    \label{eq:CoMa_helper1}
    &\bigg(
        \frac{\partial q_{01}}{\partial\gamma}
        +
        \frac{\partial q_{10}}{\partial\gamma}
    \bigg)^2
    \cdot
    \bigg[
        \frac{e^{\frac{1}{2}(1-p)^{2K}(1-q_{01}-q_{10})^2}+1}{e^{\frac{1}{2}(1-p)^{2K}(1-q_{01}-q_{10})^2}-1}
        \\\nonumber
        &\ \ \ \ \ 
        \cdot(1-p)^{2K}(1-q_{01}-q_{10})^2
        -
        1
    \bigg]
    \geq
    \\\nonumber
    &\ \ \ \ 
    (1-q_{01}-q_{10})
    \bigg(
        -
        \frac{\partial^2 q_{10}}{\partial\gamma^2}    
        -
        \frac{\partial^2 q_{01}}{\partial\gamma^2}
    \bigg)
\end{align}
The LHS of (\ref{eq:CoMa_helper1}) is non-negative (as $\frac{e^{0.5x}+1}{e^{0.5x}-1}\cdot x\geq 4$).
The RHS is a multiplication of a non-negative term with a non-positive one:
\begin{align}
    -\frac{\partial^2 q_{10}}{\partial\gamma^2}
    &=
    \sum_{j=1}^K
    \binom{K}{j}\frac{p^j (1-p)^{K-j}}{1-(1-p)^K}
    \cdot
    \frac{\exp\big\{\frac{-\gamma_1}{j\rho +1}\big\}}{(j\rho +1)^2}
    \\
    \frac{\partial^2 q_{01}}{\partial\gamma^2}
    &=
    e^{-\gamma}
    =
    \sum_{j=1}^K
    \binom{K}{j}\frac{p^j (1-p)^{K-j}}{1-(1-p)^K}
    \cdot
    e^{-\gamma}
\end{align}
\normalsize
Hence:
\begin{align}
    \label{eq:CoMa_helper2}
    \bigg(
        -
        \frac{\partial^2 q_{10}}{\partial\gamma^2}    
        -
        \frac{\partial^2 q_{01}}{\partial\gamma^2}
    \bigg)
    &=
    \sum_{j=1}^K
    \binom{K}{j}\frac{p^j (1-p)^{K-j}}{1-(1-p)^K}
    \\\nonumber
    &\ \ \ \ 
    \cdot
    \bigg(
        \frac{\exp\big\{\frac{-\gamma_1}{j\rho +1}\big\}}{(j\rho +1)^2}
        -
        e^{-\gamma}
    \bigg)
\end{align}
This is a weighted sum of elements of the forms:
\begin{align}
    \label{eq:CoMa_helper_rho_view}
    \frac{e^{-\frac{a}{x+1}}}{(x+1)^2}-e^{-a}
    \\
    \label{eq:CoMa_helper_gamma_view}
    \frac{e^{-\frac{x}{a+1}}}{(a+1)^2}-e^{-x}
\end{align}
Where (\ref{eq:CoMa_helper_rho_view}) describes the difference as a function of $\rho$ and (\ref{eq:CoMa_helper_gamma_view}) describes it as a function of $\gamma$.
In both cases, if $a\geq0$, the terms are non-positive.
In other words, (\ref{eq:CoMa_helper1}) is always true so the objective function is convex in $\gamma$.
\end{proof}

\begin{proof}[Proof of Theorem \ref{theo:CoMa_b_opt_prob_equiv}]
We shall invoke the KKT conditions.
Lemma \ref{eq:CoMa_b_opt_prob_orig_reduce_weak_ineq} proves that all Lagrange Multipliers are nulled except for the multiplier of the constraint $p\leq \frac{1}{2}$, or equivalently $\alpha\leq \frac{K}{2}$ (Complementary Slackness).
Hence, the Lagrangian's gradient is:
\begin{align}
    \nabla L(\gamma, p, \lambda)
    = 
    \begin{bmatrix}
        \frac{\partial \beta}{\partial \gamma}
        \\
        \frac{\partial \beta}{\partial p} + \lambda
    \end{bmatrix}
    =
    \underline{0}
\end{align}
If $\lambda \neq 0$, then $p=\frac{1}{2}$, and $\gamma^* = \gamma_2$.
If $\lambda = 0$, then $p\in(0,\frac{1}{2})$.
According to corollary \ref{cor:CoMa_gamma1_opt} $\lambda = 0$, so $(\gamma^*, p^*)$ must be an interior point.
Lemma \ref{lem:CoMa_obj_convex_in_gamma_suff} shows that $\gamma^*$ is unique, so the optimization problem becomes one-dimensional in $p$.
The interval $[0,0.5]$ is closed and $\beta$ is continuous, so a global minimum $p^*$ exists.
\end{proof}

\subsection{Proof of Lemma \ref{lem:beta_scale_K_inf}}
\label{appendix:proof_beta_scale_K_inf}
We note that by the famous limit $\lim_{n\to\infty}(1-\frac{x}{n})^n = e^{-x}$ we have:
\begin{align}
    \label{eq:beta_scale_limit1}
    \bigg(
        1-\frac{\alpha}{K}
    \bigg)^{2K}
    \to
    e^{-2\alpha}
\end{align}
We remind that $K\cdot p = \alpha$.
Therefore, whether $\beta$ tends to a constant depends on the limit:
\begin{align}
    \lim_{K\to\infty} q_{10}
    &\underset{(a)}{=}
    \lim_{K\to\infty}\sum_{j=1}^K \binom{K}{j}\frac{p^j(1-p)^{K-j}}{1-(1-p)^K}
    \\\nonumber
    &\quad\cdot\bigg(1 - \exp\bigg\{\frac{-\gamma}{j \cdot \rho + 1}\bigg\}\bigg)
    \\
    &\underset{(b)}{=}
    1-\lim_{K\to\infty}\sum_{j=1}^K \binom{K}{j}\frac{p^j(1-p)^{K-j}}{1-(1-p)^K}
    \\\nonumber
    &\quad\cdot\exp\bigg\{\frac{-\gamma}{j \cdot \rho + 1}\bigg\}
    \\
    &\underset{(c)}{=}
    1-\lim_{K\to\infty}\frac{1}{1-(1-p)^K}
    \\\nonumber
    &\quad\cdot\lim_{K\to\infty}\sum_{j=1}^K \binom{K}{j}p^j(1-p)^{K-j}\exp\bigg\{\frac{-\gamma}{j \cdot \rho + 1}\bigg\}
    \\\label{eq:beta_scale_limit2}
    &\underset{(d)}{=}
    1-\frac{1}{1-e^{-\alpha}}\cdot\sum_{j=1}^\infty e^{-\alpha}\frac{\alpha^j}{j!}\exp\bigg\{\frac{-\gamma}{j \cdot \rho + 1}\bigg\}
\end{align}
Where step (a) replaced $q_{10}$ with its exact expression from Theorem \ref{eq:CharaErr_q10}.
Steps (b) and (c) used the Limit Sum and Product Laws, respectively.
The final step, (d), used Poisson Limit Theorem and the famous limit.
\\
Combining (\ref{eq:beta_scale_limit1}) and (\ref{eq:beta_scale_limit2}) with Theorem \ref{theo:CoMa_b_opt_prob_equiv} when $K\to\infty$ results in an optimization problem independent of $K$ (or $N$), completing the proof.

\subsection{Proof of Corollary \ref{lem:beta_scale_rho}}
\label{appendix:proof_beta_scale_rho}
When $\rho\to0$, the exponents in Theorem \ref{eq:CharaErr_q10} tend to $e^{-\gamma}$.
Hence, $q_{10}\to 1-q_{01}$ when $\rho\to 0$, resulting in $\beta\to\infty$.
When $\rho\to\infty$, the exponents in Theorem \ref{eq:CharaErr_q10} tend to 1, so $q_{10}\to0$.
Since the rest of the parameters are unaffected by $\rho$, $\beta$'s limit is a constant (with respect to $\rho$).

\subsection{Proof of Theorem \ref{eq:ConverseMrBound}}
\label{appendix:proof_ConverseMrBound}
Denote $\underline{\tilde{Y}}$ as the noiseless $\underline{Y}$.
It is the column-wise Boolean sum of the $K$ transmitted codewords.
Let $\mathcal{W}\in\{1,2,\dots,\binom{N}{K}C^K\}$ be the index of the set corresponding to the $K$ messages transmitted.
The codewords corresponding to $\mathcal{W}$ are $\mathcal{C}(\mathcal{W})$.
Observe that we can treat $\underline{Y}$ as an output of some discrete channel (characterized by $q_{10}$ and $q_{01}$) whose input is $\underline{\tilde{Y}}$.
Notice the following Markov Chain:
\begin{align}
    \mathcal{W}\rightarrow\mathcal{C}(\mathcal{W})\rightarrow\underline{\tilde{Y}}\rightarrow \underline{Y}\rightarrow\mathcal{\hat{C}}(\hat{\mathcal{W}})\rightarrow \mathcal{\hat{W}}
\end{align}
I.e., the $K$ messages, their corresponding codewords, the "clean" Boolean sum, the noisy output vector, the estimated codewords, and estimated messages form a Markov Chain.
Using the definition of mutual information, we have:
\begin{align}
    \label{eq:ConverseEntropyB4Fano}
    H(\mathcal{W}) = H(\mathcal{W}|\hat{\mathcal{W}}) + I(\mathcal{W}; \mathcal{\hat{\mathcal{W}}})
\end{align}
We assume we have no prior information on the messages or users, so $\mathcal{W}$ is uniform on $\{1,2,\dots \binom{N}{K}C^K\}$.
This is equivalent to $H(\mathcal{W}) = \log\binom{N}{K}C^K$.
Using Fano's Inequality, we have:
\begin{align}
    \label{eq:ConverseFano}
    H(\mathcal{W}|\mathcal{\hat{W}}) \leq 1+p_e\cdot \log\binom{N}{K}C^K
\end{align}
We have the following chain of inequalities:
\begin{align}
    I(\mathcal{W}; \mathcal{\hat{\mathcal{W}}})
    &\underset{(a)}{\leq}
    I(\underline{\tilde{Y}}; \underline{Y})
    \\
    &=
    H(\underline{Y}) - H(\underline{Y}|\underline{\tilde{Y}})
    \\
    &\underset{(b)}{=}
    H(\underline{Y}) - \sum_{m=1}^{M_r} H([\underline{Y}]_m|[\underline{Y}]_1,\dots,[\underline{Y}]_{m-1},\underline{\tilde{Y}})
    \\
    &\underset{(c)}{=}
    \sum_{m=1}^{M_r} H([\underline{Y}]_m) - \sum_{m=1}^{M_r} H([\underline{Y}]_m|[\underline{\tilde{Y}}]_m)
    \\
    &=
    \sum_{m=1}^{M_r} \big[ H([\underline{Y}]_m) - H([\underline{Y}]_m|[\underline{\tilde{Y}}]_m) \big]
    \\
    &=
    \sum_{m=1}^{M_r} I([\underline{\tilde{Y}}]_m; [\underline{Y}]_m)
    \\\label{eq:ConverseMutInfoUpBound}
    &\leq 
    M_r\cdot C_{BAC} (q_{01},q_{10})
\end{align}
(a) is valid due to the Data Processing Inequality.
In (b), we have used the Entropy Chain Rule, whereas in (c), we used the fact that $[\underline{\tilde{Y}}]_m$ ($[\underline{Y}]_m$) is independent of $[\underline{\tilde{Y}}]_k$ ($[\underline{Y}]_k$) for all $m\neq k$.
Now, we can put (\ref{eq:ConverseMutInfoUpBound}) and (\ref{eq:ConverseFano}) into (\ref{eq:ConverseEntropyB4Fano}):
\begin{align}
    \nonumber
    \log \binom{N}{K}C^K
    &\leq
    1 + p_e\cdot \log \binom{N}{K}C^K
    % \\
    % &
    + M_r\cdot C_{BAC} (q_{01},q_{10})
\end{align}
Rearranging both sides results in the following:
\begin{align}
    M_r \geq \frac{(1-p_e)\cdot \log \binom{N}{K}C^K-1}{C_{BAC} (q_{01},q_{10})}
\end{align}
Using Stirling's Approximation:
\begin{align}
    \log \binom{N}{K}C^K
    &=
    \log \binom{N}{K}
    +
    \log C^K
    \\
    &\approx
    K\log \frac{N}{K}
    +
    K\log C
    \\
    &=
    K\log \frac{N}{K}\cdot C
\end{align}
Which results in the following:
\begin{align}
    M_r \geq \frac{(1-p_e)\cdot K\log \frac{N\cdot C}{K}}{C_{BAC} (q_{01},q_{10})}
\end{align}
