# Supplementary material for: Order-optimal Joint Transmission and Identification in Massive Multi-User MIMO via Group Testing
Source: arXiv:2210.00421 source file (2023-01-18)
Supplement: Supplementary file 3 [file Proofs_tmp.tex]

\subsection{Proof of Theorem \ref{theo:CoMa_b_opt_prob_equiv}}
\label{appendix:proof_CoMa_b_opt_prob_equiv}
First, we simplify $\frac{p_0}{q_{10}}-1$:
\begin{align}
    \nonumber
    \frac{p_0}{q_{10}} -1
    &=
    \frac{(1-p)^K (1-q_{01}) + (1-(1-p)^K)q_{10}}{q_{10}} - 1
    \\\label{eq:CoMa_Delta_up_simp}
    &=
    (1-p)^K\cdot\frac{1-q_{01}-q_{10}}{q_{10}}
\end{align}
Now, we convert the problem in (\ref{eq:CoMa_b_opt_prob_orig}) to a minimization problem by removing the dependence on $\Delta$: 
\begin{lemma}
\label{eq:CoMa_b_opt_prob_orig_reduce_minimax}
The objective function in (\ref{eq:CoMa_b_opt_prob_orig}) can be re-written as follows:
\begin{align}
    \nonumber
    \frac{(1+\delta)\ln 2}{\alpha\big(1-\exp\{-\frac{1}{2}(1-p)^{2K}(1-q_{10}-q_{01})^2\}\big)}
\end{align}
\end{lemma}
\begin{proof}
Derive $\beta_i$ by $\Delta$:
\begin{align}
    \frac{\partial\beta_1}{\partial \Delta}
    &=
    -\frac{4 q_{10}^2 e^{-2(q_{10}\Delta)^2}\Delta}{(\cdot)^2} \leq 0 \ \forall \Delta\geq0
    \\
    \frac{\partial\beta_2}{\partial \Delta}
    &=
    \frac{4q_{10}e^{-2(p_0-q_{10}(\Delta+1))^2}(p_0-q_{10}(\Delta+1))}{(\cdot)^2}
\end{align}
The last term is non-negative as long as $\Delta\leq \frac{p_0}{q_{10}}-1$.
Hence, $\beta_1$ decrease with $\Delta$ whereas $\beta_2$ increase in $\Delta$.
In other words, the minimax problem would pick the equalizer:
\begin{align}
    \Delta^*
    &=
    \frac{1}{2}\bigg(\frac{p_0}{q_{10}}-1\bigg)
\end{align}
Putting $\Delta^*$ and (\ref{eq:CoMa_Delta_up_simp}) back into $\beta_1=\beta_2$ results in the following term inside the exponent:
\begin{align}
    q_{10}\cdot \frac{1}{2}\bigg(\frac{p_0}{q_{10}}-1\bigg)
    &=
    \frac{1}{2}(1-p)^K(1-q_{01}-q_{10})
\end{align}
\end{proof}
We shall henceforth name the objective function $\beta = (1+\delta)\cdot\beta(\gamma, \alpha)$.
Now, we shall prove that the solution must be an interior point of the rectangle $[0,\frac{K}{2}]\times[0,\infty)$:
\begin{lemma}
\label{eq:CoMa_b_opt_prob_orig_reduce_weak_ineq}
All strong inequalities in (\ref{eq:CoMa_b_opt_prob_orig}) can be written with weak inequalities.
\end{lemma}
\begin{proof}
We'll show that each time some variable meets its inequality, then either $\beta_1\to\infty$ or $\beta_2\to\infty$.
When $\gamma = 0$, $q_{10} = 0$ and $\beta_1\to\infty$.
The same occurs when $\Delta = 0$.
When $\Delta = \frac{p_0}{q_{10}}-1$ then $\beta_2\to\infty$.
When $\alpha = 0$ both $\beta_i\to\infty$.
Hence, we can replace the strong inequalities with weak inequalities as we do not introduce new solutions to the optimization problem.
\end{proof}
We are left with proving that $\alpha = \frac{K}{2}$ is not a solution to the optimization problem.
To do this, we show that there always is an interior point with a lower objective value.
Hence, we define the following two quantities:

\begin{definition}
\label{def:CoMa_gamma1}
For any fixed $p$, we define $\gamma_1$ to be the solution to:
\begin{align}
    \nonumber
    e^{-\gamma}
    =
    \sum_{j=1}^K \binom{K}{j}\frac{p^j (1-p)^{K-j}}{1-(1-p)^K}
    \cdot 
    \frac{\exp\big\{\frac{-\gamma}{j\rho +1}\big\}}{j\rho +1}
\end{align}
\end{definition}

\begin{definition}
\label{def:CoMa_gamma2}
Let $\gamma_2$ be the solution to:
\begin{align}
    \nonumber
    e^{-\gamma}
    =
    \sum_{j=1}^K \binom{K}{j}\frac{1}{2^K-1}\cdot\frac{\exp\big\{\frac{-\gamma}{j\rho +1}\big\}}{j\rho +1}
\end{align}
\end{definition}
We want to show that $\gamma_1$, as an interior point, has a lower objective function than $\gamma_2$, a point on the boundary.

\begin{lemma}
\label{lem:CoMa_beta_trend_gamma1}
$\beta(\gamma_1)$ is increasing in $\gamma_1$, where $\gamma_1$ is as defined in definition \ref{def:CoMa_gamma1}.
\end{lemma}

\begin{proof}
Putting $\gamma_1$ in $g(\gamma,p)\triangleq(1-q_{01}-q_{10})$ yields:
\begin{align}
    g(\gamma_1,p)
    &=
    1
    -
    \sum_{j=1}^K
    \binom{K}{j}\frac{p^j (1-p)^{K-j}}{1-(1-p)^K}
    \cdot
    \bigg(
        \\\nonumber
        &\ \ \ \ 
        \frac{\exp\big\{\frac{-\gamma_1}{j\rho +1}\big\}}{j\rho +1}
        +1-
        \exp\bigg\{-\frac{\gamma_1}{j \rho + 1}\bigg\}
    \bigg)
    \\
    &=
    \sum_{j=1}^K
    \binom{K}{j}\frac{p^j (1-p)^{K-j}}{1-(1-p)^K}
    \cdot
    \frac{j\rho\cdot \exp\big\{\frac{-\gamma_1}{j\rho +1}\big\}}{j\rho +1}
\end{align}
$g(\gamma_1(p),p)$ is a sum of non-negative numbers, so $g(\gamma_1,p)\geq0$.
Furthermore, $\frac{\partial g}{\partial \gamma_1} \leq 0$.
Observe $\beta$'s derivative with respect to $\gamma_1$:
\begin{align}
    \frac{\partial\beta(\gamma_1)}{\partial\gamma_1}
    =
    -\frac{(1-p)^{2K}e^{(\cdot)} g(\gamma_1)\cdot \frac{\partial g}{\partial \gamma_1}}{\alpha\cdot (\cdot)^2} \geq 0 \ \forall\alpha > 0
\end{align}
\end{proof}

\begin{lemma}
\label{lem:CoMa_gamma1_lb}
\begin{align}
    e^{-\gamma_1}
    \geq
    \sum_{j=1}^K \binom{K}{j}\frac{1}{2^K-1}\cdot\frac{\exp\big\{\frac{-\gamma_1}{j\rho +1}\big\}}{j\rho +1}
\end{align}
With equality if and only if $p=0.5$.
\end{lemma}

\begin{proof}
Observing $\gamma_1 = \gamma_1(p)$, we have $\gamma_2 = \gamma_1(0.5)$.
\begin{align}
    e^{-\gamma_1}
    &\underset{(a)}{=}
    \sum_{j=1}^K \binom{K}{j}\frac{p^j (1-p)^{K-j}}{1-(1-p)^K}
    \cdot 
    \frac{\exp\big\{\frac{-\gamma_1}{j\rho +1}\big\}}{j\rho +1}
    \\
    &\underset{(b)}{=}
    \sum_{j=\floor{\frac{K-1}{2}}}^K \binom{K}{j}\frac{p^j (1-p)^{K-j}}{1-(1-p)^K}
    \cdot 
    \frac{\exp\big\{\frac{-\gamma_1}{j\rho +1}\big\}}{j\rho +1}
    \\\nonumber
    &\ \ \ \ +
        \sum_{j=1}^{\floor{\frac{K-1}{2}}-1} \binom{K}{j}\frac{p^j (1-p)^{K-j}}{1-(1-p)^K}
        \cdot 
        \frac{\exp\big\{\frac{-\gamma_1}{j\rho +1}\big\}}{j\rho +1}
    \\
    &\underset{(c)}{\geq}
    \sum_{j=\floor{\frac{K-1}{2}}}^K \binom{K}{j}\frac{1}{2^K-1}
    \cdot 
    \frac{\exp\big\{\frac{-\gamma_1}{j\rho +1}\big\}}{j\rho +1}
    \\\nonumber
    &\ \ \ \ +
        \sum_{j=1}^{\floor{\frac{K-1}{2}}-1} \binom{K}{j}\frac{p^j (1-p)^{K-j}}{1-(1-p)^K}
        \cdot 
        \frac{\exp\big\{\frac{-\gamma_1}{j\rho +1}\big\}}{j\rho +1}    
    \\
    &\underset{(d)}{=}
    \sum_{j=1}^K \binom{K}{j}\frac{1}{2^K-1}
    \cdot 
    \frac{\exp\big\{\frac{-\gamma_1}{j\rho +1}\big\}}{j\rho +1}
    \\\nonumber
    &\ \ \ \ +
        \sum_{j=1}^{\floor{\frac{K-1}{2}}-1} \binom{K}{j}\bigg(\frac{p^j (1-p)^{K-j}}{1-(1-p)^K}
        -
        \frac{1}{2^K-1}
        \bigg)
        \\\nonumber
        &\quad\quad\cdot
        \frac{\exp\big\{\frac{-\gamma_1}{j\rho +1}\big\}}{j\rho +1}
    \\
    &\underset{(e)}{\geq}
    \sum_{j=1}^K \binom{K}{j}\frac{1}{2^K-1}
    \cdot 
    \frac{\exp\big\{\frac{-\gamma_1}{j\rho +1}\big\}}{j\rho +1}
\end{align}
In (a), we used definition \ref{def:CoMa_gamma1}.
We separated the sum in (b) and used $p$'s limited range ($p\in[0,1]$) in (c).
We have added and subtracted the same term in (d), whereas in (e), we discarded non-negative terms due to $p$'s range.
If $\gamma_1 = \gamma_2$, then we have equality from definition \ref{def:CoMa_gamma2}.
\end{proof}

\begin{corollary}
\label{cor:CoMa_gamma1_opt}
$\beta(\gamma_2)\geq\beta(\gamma_1)$
\end{corollary}

\begin{proof}
$\gamma_2$ is the maximizer of the lower bound in lemma \ref{lem:CoMa_gamma1_lb}.
In other words:
\begin{align}
    e^{-\gamma_1} \geq e^{-\gamma_2}
\end{align}
By taking $\ln(\cdot)$ from both sides, we have $\gamma_2\geq\gamma_1$.
Using lemma \ref{lem:CoMa_beta_trend_gamma1} gives us the desired result.
\end{proof}

Now, after showing that the solution must be an interior point, we are ready to show that a solution exists:
\begin{lemma}
\label{lem:CoMa_obj_convex_in_gamma_suff}
The objective function in lemma \ref{eq:CoMa_b_opt_prob_orig_reduce_minimax} is convex in $\gamma$.
\end{lemma}

\begin{proof}
$\beta(\gamma)$ is convex in $\gamma$ if and only if:
\begin{align}
    2\bigg(\frac{\partial f}{\partial\gamma}\bigg)^2
    -
    f(\gamma)\cdot\frac{\partial^2 f}{\partial\gamma^2}
    \geq
    0
\end{align}
By dividing by non-zero positive quantities, the above condition is simplified to:
\begin{align}
    \label{eq:CoMa_b_convex_gamma_cond}
    &\bigg(
        e^{\frac{1}{2}(1-p)^{2K}(1-q_{01}-q_{10})^2}+1
    \bigg)
    \cdot
    (1-p)^{2K}
    \cdot
    (1-q_{01}-q_{10})^2
    \\\nonumber
    &\ \ \ \ 
    \cdot
    \bigg(
        \frac{\partial q_{01}}{\partial\gamma}
        +
        \frac{\partial q_{10}}{\partial\gamma}
    \bigg)^2
    +
    \bigg(
        e^{\frac{1}{2}(1-p)^{2K}(1-q_{01}-q_{10})^2}-1
    \bigg)
    \\\nonumber
    &\ \ \ \ 
    \cdot
    \bigg[
        (
            1
            -
            q_{01}
            -
            q_{10}
        )
        \bigg(
            \frac{\partial^2 q_{01}}{\partial\gamma^2}
            +
            \frac{\partial^2 q_{10}}{\partial\gamma^2}
        \bigg)
        \\\nonumber&\quad
        -
        \bigg(
            \frac{\partial q_{01}}{\partial\gamma}
            +
            \frac{\partial q_{10}}{\partial\gamma}
        \bigg)^2
    \bigg]
    \geq 0
\end{align}
Rearranging both sides results in the following:
\begin{align}
    \label{eq:CoMa_helper1}
    &\bigg(
        \frac{\partial q_{01}}{\partial\gamma}
        +
        \frac{\partial q_{10}}{\partial\gamma}
    \bigg)^2
    \cdot
    \bigg[
        \frac{e^{\frac{1}{2}(1-p)^{2K}(1-q_{01}-q_{10})^2}+1}{e^{\frac{1}{2}(1-p)^{2K}(1-q_{01}-q_{10})^2}-1}
        \\\nonumber
        &\ \ \ \ \ 
        \cdot(1-p)^{2K}(1-q_{01}-q_{10})^2
        -
        1
    \bigg]
    \geq
    \\\nonumber
    &\ \ \ \ 
    (1-q_{01}-q_{10})
    \bigg(
        -
        \frac{\partial^2 q_{10}}{\partial\gamma^2}    
        -
        \frac{\partial^2 q_{01}}{\partial\gamma^2}
    \bigg)
\end{align}
The LHS of (\ref{eq:CoMa_helper1}) is non-negative (as $\frac{e^{0.5x}+1}{e^{0.5x}-1}\cdot x\geq 4$).
The RHS is a multiplication of a non-negative term with a non-positive one:
\begin{align}
    -\frac{\partial^2 q_{10}}{\partial\gamma^2}
    &=
    \sum_{j=1}^K
    \binom{K}{j}\frac{p^j (1-p)^{K-j}}{1-(1-p)^K}
    \cdot
    \frac{\exp\big\{\frac{-\gamma_1}{j\rho +1}\big\}}{(j\rho +1)^2}
    \\
    \frac{\partial^2 q_{01}}{\partial\gamma^2}
    &=
    e^{-\gamma}
    =
    \sum_{j=1}^K
    \binom{K}{j}\frac{p^j (1-p)^{K-j}}{1-(1-p)^K}
    \cdot
    e^{-\gamma}
\end{align}
\normalsize
Hence:
\begin{align}
    \label{eq:CoMa_helper2}
    \bigg(
        -
        \frac{\partial^2 q_{10}}{\partial\gamma^2}    
        -
        \frac{\partial^2 q_{01}}{\partial\gamma^2}
    \bigg)
    &=
    \sum_{j=1}^K
    \binom{K}{j}\frac{p^j (1-p)^{K-j}}{1-(1-p)^K}
    \\\nonumber
    &\ \ \ \ 
    \cdot
    \bigg(
        \frac{\exp\big\{\frac{-\gamma_1}{j\rho +1}\big\}}{(j\rho +1)^2}
        -
        e^{-\gamma}
    \bigg)
\end{align}
This is a weighted sum of elements of the forms:
\begin{align}
    \label{eq:CoMa_helper_rho_view}
    \frac{e^{-\frac{a}{x+1}}}{(x+1)^2}-e^{-a}
    \\
    \label{eq:CoMa_helper_gamma_view}
    \frac{e^{-\frac{x}{a+1}}}{(a+1)^2}-e^{-x}
\end{align}
Where (\ref{eq:CoMa_helper_rho_view}) describes the difference as a function of $\rho$ and (\ref{eq:CoMa_helper_gamma_view}) describes it as a function of $\gamma$.
In both cases, if $a\geq0$, the terms are non-positive.
In other words, (\ref{eq:CoMa_helper1}) is always true, so the objective function is convex in $\gamma$.
\end{proof}

\begin{proof}[Proof of Theorem \ref{theo:CoMa_b_opt_prob_equiv}]
We shall invoke the KKT conditions.
Lemma \ref{eq:CoMa_b_opt_prob_orig_reduce_weak_ineq} proves that all Lagrange Multipliers are nulled except for the multiplier of the constraint $p\leq \frac{1}{2}$, or equivalently $\alpha\leq \frac{K}{2}$ (Complementary Slackness).
Hence, the Lagrangian's gradient is:
\begin{align}
    \nabla L(\gamma, p, \lambda)
    = 
    \begin{bmatrix}
        \frac{\partial \beta}{\partial \gamma}
        \\
        \frac{\partial \beta}{\partial p} + \lambda
    \end{bmatrix}
    =
    \underline{0}
\end{align}
If $\lambda \neq 0$, then $p=\frac{1}{2}$, and $\gamma^* = \gamma_2$.
If $\lambda = 0$, then $p\in(0,\frac{1}{2})$.
According to corollary \ref{cor:CoMa_gamma1_opt} $\lambda = 0$, so $(\gamma^*, p^*)$ must be an interior point.
Lemma \ref{lem:CoMa_obj_convex_in_gamma_suff} shows that $\gamma^*$ is unique, so the optimization problem becomes one-dimensional in $p$.
The interval $[0,0.5]$ is closed, and $\beta$ is continuous, so a global minimum $p^*$ exists.
\end{proof}

\subsection{Proof of Lemma \ref{lem:beta_scale_K_inf}}
\label{appendix:proof_beta_scale_K_inf}
We note that by the famous limit $\lim_{n\to\infty}(1-\frac{x}{n})^n = e^{-x}$ we have:
\begin{align}
    \label{eq:beta_scale_limit1}
    \bigg(
        1-\frac{\alpha}{K}
    \bigg)^{2K}
    \to
    e^{-2\alpha}
\end{align}
We remind that $K\cdot p = \alpha$.
Therefore, whether $\beta$ tends to a constant depends on the limit:
\begin{align}
    \lim_{K\to\infty} q_{10}
    &\underset{(a)}{=}
    \lim_{K\to\infty}\sum_{j=1}^K \binom{K}{j}\frac{p^j(1-p)^{K-j}}{1-(1-p)^K}
    \\\nonumber
    &\quad\cdot\bigg(1 - \exp\bigg\{\frac{-\gamma}{j \cdot \rho + 1}\bigg\}\bigg)
    \\
    &\underset{(b)}{=}
    1-\lim_{K\to\infty}\sum_{j=1}^K \binom{K}{j}\frac{p^j(1-p)^{K-j}}{1-(1-p)^K}
    \\\nonumber
    &\quad\cdot\exp\bigg\{\frac{-\gamma}{j \cdot \rho + 1}\bigg\}
    \\
    &\underset{(c)}{=}
    1-\lim_{K\to\infty}\frac{1}{1-(1-p)^K}
    \\\nonumber
    &\quad\cdot\lim_{K\to\infty}\sum_{j=1}^K \binom{K}{j}p^j(1-p)^{K-j}\exp\bigg\{\frac{-\gamma}{j \cdot \rho + 1}\bigg\}
    \\\label{eq:beta_scale_limit2}
    &\underset{(d)}{=}
    1-\frac{1}{1-e^{-\alpha}}\cdot\sum_{j=1}^\infty e^{-\alpha}\frac{\alpha^j}{j!}\exp\bigg\{\frac{-\gamma}{j \cdot \rho + 1}\bigg\}
\end{align}
Where step (a) replaced $q_{10}$ with its exact expression from Theorem \ref{eq:CharaErr_q10}.
Steps (b) and (c) used the Limit Sum and Product Laws, respectively.
The final step, (d), used Poisson Limit Theorem and the famous limit.
\\
Combining (\ref{eq:beta_scale_limit1}) and (\ref{eq:beta_scale_limit2}) with Theorem \ref{theo:CoMa_b_opt_prob_equiv} when $K\to\infty$ results in an optimization problem independent of $K$ (or $N$), completing the proof.
